# Supplementary material for: Machine Translation of Mathematical Text
Source: arXiv:2010.05229 ancillary file (2020-10-11)
Supplement: Supplementary file 1 [file Ohri2020_PolyMath_preprint-fr.pdf]

# Machine Translation of Mathematical Text

Aditya Ohri and Tanya Schmah

October 9, 2020

## 1 introduction

La traduction automatique pour des domaines spécialisés tels que le texte juridique ou médical a reçu une attention considérable. Les progrès dans ces domaines ont été utiles dans la pratique et ont également donné lieu à de nouvelles techniques dans des domaines tels que l'adaptation de domaine.[3], extraction automatique de termes[19] et des approches sensibles au domaine de la traduction automatique à usage général [1]. Dans le présent article, nous considérons le domaine du texte mathématique, tel qu'il a été produit par des chercheurs en mathématiques et domaines connexes, et par des enseignants de niveau post-secondaire de ces matières. Pour clarifier, nous considérons le langage naturel spécialisé sur les mathématiques, que nous pouvons appeler l'écriture mathématique informelle (par si hautement technique), pour le distinguer des mathématiques formelles écrites dans le langage de la logique pure. En particulier, le présent article examine le problème de la traduction de l'écriture mathématique de l'anglais vers le français. Le choix spécifique de la paire de langues est motivé par le contexte canadien particulier des auteurs. Le domaine du texte mathématique n'a, à notre connaissance, pas encore fait l'objet de recherches en traduction automatique, au-delà de quelques travaux très anciens[10][13], bien que nous mentionnions des recherches approfondies en cours dans les domaines connexes de l'ontologie mathématique et de la sémantique[25]et traduction de l'écriture mathématique informelle en mathématiques formelles [23].

Le texte mathématique présente plusieurs caractéristiques intéressantes pour le chercheur. Il mélange souvent le langage naturel avec des expressions symboliques dans la même phrase, les expressions symboliques ayant une variété de rôles grammaticaux, y compris en tant que noms, pronoms ou clauses. Le texte mathématique a sa propre grammaire et conventions, par ex. « Soit  $x$  et  $y$  des entiers » ou « Considérons une fonction  $h = f + g$ . » (Voir également[17].) De façon anecdotique, l'écriture mathématique peut être à la fois plus et moins complexe que le langage naturel typique. Il est unique dans son utilisation fréquente des définitions[25], et souvent complexe dans sa description précise des relations logiques, utilisant un vocabulaire et une grammaire qui sont standard mais rares en dehors des mathématiques, de la philosophie et du droit. Bien que nous ne soyons pas au courant d'une recherche soutenant directement cette affirmation, elle est indirectement soutenue par l'étude de Yasseri et al. Sur les entrées de

Wikipédia.[26], qui a constaté que les exemples les plus complexes étudiés, mesurés par l'indice de brouillard de Gunning, étaient ceux de la philosophie et de la physique (les mathématiques n'ont pas été prises en compte). Notez que l'indice de brouillard de Gunning dépend de la longueur moyenne des phrases et de la fréquence des mots longs. En revanche, rien dans cet article n'indique que le vocabulaire réel du texte mathématique est plus large que d'habitude. Au contraire, des preuves anecdotiques suggèrent le contraire. En particulier, les auteurs ont connaissance de nombreux exemples de chercheurs en mathématiques donnant des conférences techniques compréhensibles dans des langues dans lesquelles ils ne parlent généralement pas couramment. Si cette simplicité du vocabulaire est confirmée, alors le domaine du texte mathématique offre une possibilité intrigante de traduction automatique meilleure que d'habitude dans ce domaine limité, tout en présentant des défis uniques.

Dans la pratique, il existe un grand besoin de traduction automatique de textes mathématiques, pour les chercheurs, les enseignants et les étudiants. Si les possibilités commerciales de ce domaine peuvent ne pas être aussi évidentes qu'en médecine ou en droit, il existe une large base d'utilisateurs potentiels et un très grand nombre de documents. Par exemple la base de données MathSciNet<sup>®</sup>[18] contient plus de 3,6 millions d'articles, mais tous ne sont pas en `Latexformat`, et si nous élargissons la définition du texte mathématique pour inclure des domaines mathématiquement riches tels que la physique, l'informatique et l'ingénierie, nous pouvons considérer les 1,8 million d'articles sur `learXiv.org` serveur de pré-impression, dont la plupart sont en `Latexformat`. En outre, il y a des millions d'étudiants en mathématiques avancées avec une maîtrise limitée de l'anglais qui se fient aux manuels de langue anglaise en raison du manque de traductions disponibles.

L'un des principaux obstacles à la traduction automatique d'un texte mathématique est son contenu symbolique. La grande majorité des documents mathématiques sont désormais rédigés en `Latex`, un système de préparation de documents spécifique aux mathématiques, qui prend en charge les symboles et expressions mathématiques incorporés, ainsi que des fonctionnalités de mise en page de documents. Cette ubiquité est à la fois un obstacle à la traduction via les outils existants (qui ne comprennent pas `Latexsyntax`) et une opportunité, depuis une fois le `Latex` « obstacle » est adopté, la grande majorité des le texte mathématique moderne est désormais disponible pour la traduction automatique.

Le reste de cet article est organisé comme suit. Nous décrivons les corpus et le glossaire personnalisés que nous utilisons pour la formation et les tests de modèles. Nous décrivons ensuite nos algorithmes, qui incluent `Latexanalyse` à l'aide de `pandoc`[12] et la formation d'un « Transformateur » modèle de traduction automatique neuronale[21]. Nous évaluons notre système final sur l'ensemble des documents `LaTeX` et un petit corpus de test de paires de phrases mathématiques.

## 2 Méthodes

### 2.1 Données et prétraitement

Nous avons construit un petit glossaire personnalisé de 373 termes mathématiques (mots et phrases courtes) en combinant plusieurs listes accessibles au public (y compris [16, 5]) et en ajoutant quelques termes supplémentaires.

Pour tous les modèles d'entraînement, et pour la plupart de notre validation, nous avons utilisé un corpus combiné de paires de blocs de texte alignés (principalement des phrases), appelés ci-après notre « corpus principal », composé de : un sous-ensemble de « Hansards alignés de la 36e législature du Canada » corpus [7], un sous-ensemble de l'OPUS spécifique au domaine « Wikipédia » corpus (v1.0) [24], et notre propre coutume « math » corpus dérivé principalement de plusieurs articles de recherche du deuxième auteur TS. Le premier sous-corpus était inclus pour fournir une plus grande diversité de vocabulaire, de grammaire et de style, tandis que les deux spécifiquement sur le texte mathématique. Nous décrivons maintenant chacun de ces sous-corpus.

le « Hansards alignés de la 36e législature du Canada » corpus est un corpus de morceaux de texte alignés (phrases ou fragments plus petits) extraits des documents officiels du 36e Parlement canadien, y compris les débats de la Chambre des communes et du Sénat [7]. Le corpus complet se compose de 1,28 million de paires de phrases anglais-français, contenant 33,9 millions de mots (anglais plus français). Il s'agit d'un corpus de haute qualité composé principalement de phrases complètes. Nous l'avons choisi pour sa taille et sa qualité, et aussi dans l'espoir que le matériel source contiendrait de nombreux exemples d'un style de langage formel avec une structure similaire à un texte mathématique. Après avoir supprimé les paires de phrases contenant des informations non pertinentes telles que le titre, la date et les noms des locuteurs, nous avons mélangé au hasard l'ensemble du corpus filtré, puis sélectionné 250 000 paires de phrases.

L'OPUS « Wikipédia » corpus est un corpus de phrases parallèles extraites de Wikipedia par Krzysztof Wołk et Krzysztof Marasek [24], qui fait partie du projet OPUS [20]. Le corpus complet comprend de nombreuses paires de langues, dont nous n'utilisons que la paire anglais / français, qui se compose de 803 670 paires de phrases contenant 34 millions de mots (anglais plus français). Le sujet est vaste. Afin de nous concentrer sur le texte mathématique, nous avons appliqué un filtre de sujet naïf à ce corpus : nous avons extrait les seules paires de phrases dans lesquelles la phrase anglaise contenait au moins deux termes de notre glossaire mathématique personnalisé décrit ci-dessus. Nous avons trouvé 16 767 paires de phrases satisfaisant à ce critère. Notez que le vocabulaire de cet ensemble de données réduit contient 55 474 jetons uniques, alors que la taille moyenne du vocabulaire des sous-ensembles aléatoires du même corpus, de même taille, était de 100 738 (moyenne sur 5 échantillons aléatoires).

Le corpus mathématique personnalisé se compose de 1 075 paires de phrases en anglais et en français, les phrases anglaises étant extraites de plusieurs des travaux de recherche du deuxième auteur en mathématiques. Les phrases an-

glaises ont été extraites et traduites en français à l'aide d'une première version de notre système de traduction PolyMath avec un backend API Google Translate à l'aide de notre glossaire mathématique personnalisé. Notez que ces phrases contiennent des mots symboliques mathématiques tels que « MATH66X », qui remplacent les expressions mathématiques, comme décrit dans la section suivante.

Ces trois sous-corpus ont été combinés en un corpus hétérogène contenant un total de 267 842 blocs de texte parallèle anglais-français, que nous appelons le « principale » corpus dans le reste de cet article. La plupart de les morceaux de texte sont des phrases, nous les appelons « Phrases » ci-après, par la suite. Chaque paire de phrases du corpus principal a été segmentée par mot pour garantir que tous les jetons d'une phrase, y compris la ponctuation, étaient séparés par un espace et traités individuellement pendant la formation. Nous avons mélangé au hasard le corpus principal, puis divisé au hasard les paires de textes en ensembles d'apprentissage (80%), de validation (10%) et de test (10%).

Pour des tests supplémentaires, nous avons utilisé un autre corpus personnalisé, le « code linéaire » corpus, contenant 160 paires de phrases, extraites de notes de cours de mathématiques préparées par M. Nevins sur des codes correcteurs d'erreurs linéaires, un sujet qui n'apparaissait pas dans notre corpus principal. En commençant par des phrases françaises extraites du document source à l'aide de PolyMath, avec des expressions mathématiques tokenisées comme expliqué ci-dessus, nous les avons traduites en anglais à l'aide de Google Translate avec notre glossaire mathématique personnalisé, puis les avons relues et effectué des corrections manuelles.

## 2.2 Méthodes d'analyse

Nous utilisons une conception modulaire qui dissocie leLatexaspects d'analyse et de traduction automatique. La première tâche consiste à analyser leLatexdocumenter et extraire tout le texte en langage naturel pour la traduction tout en préservant une structure de document suffisante etLatexcommandes pour reconstruire un document complet. La deuxième tâche, abordée dans la section suivante, est de traduire le texte extrait en langue naturelle en français.

Pour la première tâche d'analyse duLatexdocument, notre outil principal était le Pandoc Universal Document Converter[12], en utilisant le wrapper Pythonpy pandoc. Pour nos besoins, puisque nous visons à traduire un anglaisLatexdocument en français tout en préservant l'originalLatexautant que possible, nous sommes « conversion » un document deLatexàLatex. Notre objectif est de tirer parti d'une représentation de document intermédiaire interne à Pandoc, le format JSON *arbre de syntaxe abstraite (AST)*, et un mécanisme pour effectuer des opérations sur cet arbre de syntaxe : les filtres pandoc, implémentés à l'aide du package Pythonpandocfilters. L'arbre de syntaxe abstraite est organisé par éléments de bloc, tels que des paragraphes, des listes à puces et des tableaux, chacun contenant une liste de « éléments en ligne » y compris des chaînes de mots individuels, des espaces et des mathématiques. Puisque les

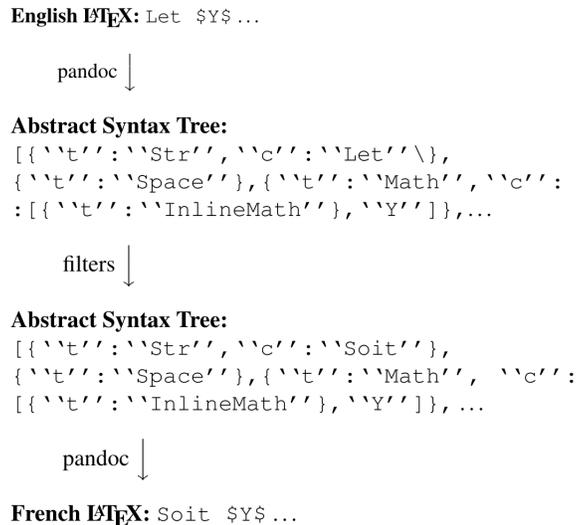

FIGURE 1 – Flux de données du module d’analyse LaTeX utilisant le convertisseur de documents universel pandoc. La représentation interne est l’*arbre syntaxique abstrait* (AST) qui est au format JSON.

filtres s’intègrent dans le PandocLatex-à-Latexconversion de fichier, l’ensemble du processus de traduction s’exécute avec un seul appel une fonction Pandoc. Un aperçu du processus est présenté ici :

Nous utilisons deux filtres pandoc, dont chacun modifie l’arbre de syntaxe abstraite. La première « coeur » Filtre Pandoc traduit tous les éléments de bloc contenant du texte en langage naturel, en joignant des chaînes de texte et des symboles mathématiques dans des phrases entières (ou parfois des phrases, comme dans les titres), en traduisant ces phrases (voir section suivante), et remettre les phrases traduites dans l’arbre de syntaxe abstraite. Notez que la structure à plus grande échelle basée sur des blocs du document est conservé dans l’arborescence de syntaxe abstraite.

En règle générale, les filtres pandoc agissent sur des éléments en ligne individuels tels que des chaînes. Cependant, pour la traduction de texte, cela est très limité, car chaque chaîne contenant un jeton individuel devrait être traduite séparément, au lieu d’une phrase entière. Ainsi, nous avons combiné ces éléments en ligne en phrases entières. Nous avons accompli cela dans un « jonction de cordes » une fonction composée de deux couches : manipulation d’éléments de bloc individuels via l’interface pandoc, et manipulation ultérieure des éléments en ligne directement. Surtout, nous incluons des formules mathématiques (en ligne ou affichées) dans nos phrases, tokenisé en « MATH » jetons de la forme « MATH<sub>n</sub>X » , où n est l’indice du jeton pour une récupération ultérieure de sa

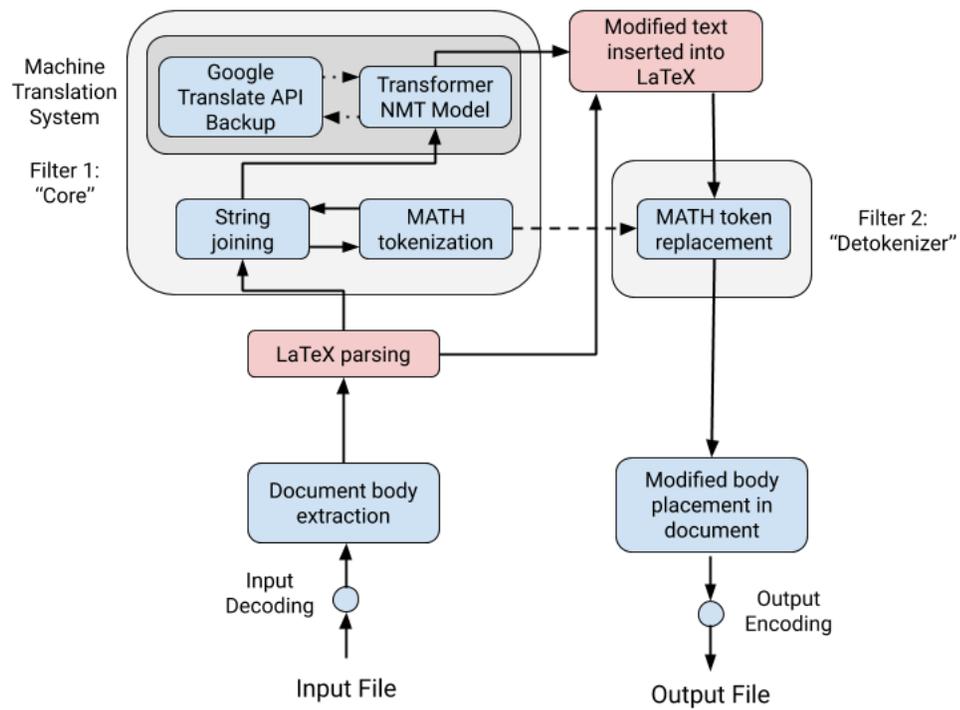

FIGURE 2 – Présentation de PolyMath Translator. Les modules de couleur rose sont implémentés à l’aide du convertisseur de documents universel pandoc, voir également Fig.1.

formule mathématique correspondante. Les formules d'origine sont enregistrées dans un objet JSON avec leur nom de jeton correspondant comme clé. De cette façon, des phrases complètes contenant ces formules peuvent être traduites sans perte de contexte environnant important.

Par exemple, considérons une phrase mathématique simpleLatex : « Soit  $Y$  la moyenne  $\mu$  et la variance  $\sigma^2$ , et un p.d.f inconnu.  $p_Y$  qui est partout différent de zéro. » Dans un bloc de paragraphe structuré JSON, cette phrase serait représentée sous la forme d'une liste d'éléments en ligne, dont le début est illustré à la Fig.1. Sans manipuler les formules mathématiques dans cette phrase, la phrase serait divisée par ces objets, de sorte que les plus grandes phrases concaténées possibles pour la traduction seraient « Laisser » , « avoir méchant » , « et variance » , etc. Après la tokenisation « math » objets, la phrase entière est concaténée en un seul « Str » élément : [ « t » : « Str » , « c » : « Soit  $Y$  la moyenne  $\mu$  et la variance  $\sigma^2$ , et un p.d.f inconnu.  $p_Y$  qui est partout différent de zéro. » ] Le format des jetons mathématiques est tel qu'ils sont traités comme des mots anglais inconnus par le (s) module (s) de traduction, et laissé inchangé dans les phrases traduites. Les expressions mathématiques peuvent désormais être traitées comme des jetons individuels lors de la traduction, et la phrase entière peut être traduite, optimisant ainsi la qualité de la traduction. Notez qu'après l'exécution du filtre, pandoc convertit automatiquement le « Str » objet de phrase de nouveau dans l'individu « Str » mot et « Espace » objets, comme dans l'arbre de syntaxe abstrait original.

Une fois que tout le texte en langage naturel dans le modifiéLatexle document a été traduit en français, il reste à remplacer le « MATH » jetons avec les formules mathématiques originales, en utilisant l'objet JSON enregistré créé par le « coeur » filtre pandoc. Ceci est accompli par un deuxième filtre pandoc appelé le « détokenizer » .

Enfin, pandoc crée un nouveau fichier LaTeX en utilisant le texte traduit et la structure du document original. L'ensemble du processus est représenté sur la Fig.2. Notez que certaines modifications apportées aux commandes LaTeX sont introduites à la suite de pandoc arbre de syntaxe abstrait ne pouvant pas représenter complètement toutes les commandes LaTeX. Cependant, lorsque les documents originaux et traduits sont compilés au format PDF, très peu de différences de format sont observées.

## 2.3 Méthodes de traduction

Pour la traduction de texte, nous avons formé un modèle de traduction automatique neuronale (NMT) personnalisé à l'aide de l'architecture Transformer pour la transduction de séquence neurale introduite par Vaswani et al.[21]. Le transformateur est un modèle de transduction de séquence neurale, c'est-à-dire un « séquence à séquence » traducteur implémenté à l'aide d'un réseau neuronal qui sort, pour toute position  $t$  dans la séquence de sortie  $y$ , une distribution conditionnelle  $p(y_t|y_{<t}, x)$  basé sur la séquence d'entrée entière  $x$  et les sorties précédentes  $y_{<t}$ . Comme la plupart des autres modèles de ce type, le Transformer dispose d'un encodeur-décodeur structure. *Attention*mécanismes

appliquent des poids aux éléments de la séquence d’entrée, qui varie en fonction de la position  $t$  dans la séquence de sortie. Cela permet au réseau de « Faites attention » certaines entrées, par exemple lors de la production du premier mot de une phrase de sortie, le réseau peut accorder le plus d’attention au premier mot de la phrase d’entrée. La principale caractéristique distinctive du modèle Transformer est son utilisation de l’auto-attention multi-têtes qui lui permet de visualiser la séquence d’entrée de différent « points de vue » en appliquant plusieurs fonctions d’attention parallèles. Par exemple, lors de l’encodage du mot « frappé » dans la phrase « J’ai frappé le ballon » , on peut accorder plus d’attention à la « je » ou la « Balle » , correspondant à la pose des questions\*à « qui a réalisé l’action ? » ou « qu’est-ce qui a été frappé ? » . Dans cet exemple de jouet, le premier point de vue serait aide le plus à conjuguer le verbe de sortie correspondant, tandis que point de vue aiderait le plus à traduire la racine du verbe. Une caractéristique clé du mécanisme d’attention Transformer est qu’il est hautement parallélisable, permettant un entraînement beaucoup plus rapide que les précédents modèles comparables. Nous avons formé un transformateur « modèle de base » tel que mis en œuvre dans OpenNMT[8], en utilisant le sous-ensemble de formation du corpus principal décrit ci-dessus. Les détails de la formation sont donnés dans la section suivante.

La sortie de notre modèle de transformateur formé est déjà de haute qualité, comme on le verra dans la section suivante. Cependant, alors que nous pouvons nous attendre à modèle pour avoir de bonnes performances sur le texte mathématique, grâce à l’inclusion délibérée de texte mathématique dans notre ensemble de formation, nous ne pouvons pas nous attendre à ce qu’il fonctionne aussi bien sur le texte anglais général en tant que services de traduction commerciale tels que Google Translate, en raison de notre ensemble de formation limité et de notre architecture Transformer prête à l’emploi. Même les phrases mathématiques peuvent contenir des caractéristiques linguistiques non vu dans notre ensemble de formation limité. Pour cette raison, nous avons utilisé Google Traduction comme « sauvegarde » traducteur dans notre système final, comme suit.

Nous exécutons d’abord toutes les phrases via notre modèle principal Transformer. Le résultat de ce processus n’est pas simplement une phrase traduite mais aussi un score de vraisemblance conditionnelle logarithmique cumulative  $\sum_t \log p(y_t | y_{<t}, x)$ , où la somme est sur tous les jetons dans la phrase de sortie. En divisant cela par la longueur de la phrase, on obtient la moyenne loger la vraisemblance conditionnelle par jeton, qui est une mesure de confiants que le système est de sa prédiction. Ceci est généralement converti en un *perplexité* valeur, calculé comme  $\exp(-\text{mean conditional likelihood})$ , qui est le plus bas pour les prédictions les plus fiables. Par inspection visuelle de la qualité des traductions des phrases de validation, nous avons établi une valeur seuil de 2.05 pour la perplexité, au-dessous duquel nous sommes satisfaits de la qualité de la traduction. Au moment du test, chaque fois que notre modèle Transformer produit une phrase avec perplexité au-dessus de ce seuil, nous avons écarté la sortie et à la place retraduit la phrase d’entrée en utilisant le Google Translate API avec notre glossaire mathématique personnalisé.

## 2.4 Modifications LaTeX spécifiques au français

Enfin, puisque le français LaTeX a ses propres conventions typographiques, PolyMath ajoute un « français » à la classe de document et ajoute les lignes suivantes à l'en-tête du document :

```
\usepackage[T1]{fontenc}
\usepackage{babel}
```

Il traduit également explicitement tout LaTeX-style guillemets doubles (c.-à-d. deux guillemets consécutifs ou deux guillemets simples consécutifs) dans `\oget fg{}` respectivement.

## 2.5 Formation, validation et tests

Nous avons utilisé la métrique BLEU [14] pour évaluer la qualité des traductions automatiques par rapport à une traduction cible donnée. Cette métrique est standard dans le domaine et s'est avérée bien corrélée avec le jugement humain de la qualité de la traduction.

Comme indiqué précédemment, notre corpus principal a été divisé au hasard en ensembles de formation (80%), de validation (10%) et de test (10%). Le sous-ensemble de formation contient 214 272 paires de phrases anglais-français, tandis que les sous-ensembles de validation et de test contiennent chacun 26 785 paires de phrases.

Nous avons formé le modèle Transformer avec un vocabulaire de 50 000 mots sur le sous-ensemble de formation du corpus principal. Nous avons défini la taille du lot à 3072 jetons et un maximum de 100 000 étapes ou 65 époques du corpus entier pour la formation, et nous avons utilisé les valeurs par défaut de tous les autres hyperparamètres. Nous n'avons réglé aucun hyperparamètre de modèle. Nous avons utilisé une condition d'arrêt précoce, pour éviter le sur-ajustement et réduire les coûts de calcul une fois que le modèle converge, pour lequel nous avons utilisé le sous-ensemble de validation du corpus principal. La condition d'arrêt était : s'arrêter lorsque le score de validation BLEU ne s'améliore pas de plus de 0,2 point sur les 4 dernières évaluations. Après 50000 étapes ou 32 époques, notre modèle a satisfait aux critères d'arrêt précoce et a arrêté l'entraînement avec un score de validation BLEU de 28,7. Cette formation a nécessité 12 heures sur 8 GPU Tesla V100.

Pendant l'exécution, le modèle Transformer déduit d'abord la traduction d'une phrase particulière, et s'il a une perplexité de test inférieure ou égale à 2,05, cette prédiction est utilisée. Sinon, la phrase est traduite par Google Translate avec notre glossaire mathématique personnalisé, comme discuté dans la section 2.3.

Après avoir formé le modèle NMT et intégré les autres composants décrits ci-dessus, nous avons utilisé les corpus de test pour évaluer la qualité du système PolyMath. Nous comparons l'ensemble du système PolyMath Translation avec ses deux composants : le modèle NMT seul ; et Google Translate seul. Pour chaque système, un score BLEU de test pour a été calculé pour deux corpus : le

sous-ensemble de test du corpus principal multi-domaine ; et le « bloc linéaire » corpus de texte mathématique.

### 3 Résultats

Table 1 montre nos principaux résultats expérimentaux, qui sont Scores BLEU calculés sur nos deux corpus tests, pour les traductions effectuées par : le PolyMath Translator (système complet) ; Google Traduction uniquement (sans glossaire) ; et notre modèle Transformer NMT qualifié uniquement. Comme prévu, le système complet PolyMath produit de meilleurs résultats que les deux systèmes de traduction qu’il utilise. Il est également à noter que le modèle Transformer NMT a surpassé Google Traduction, pair sur du texte multi-domaine. Cela peut être en partie dû à la similitude des données d’entraînement et de test, qui a donné au modèle un avantage. Cependant, cela suggère que notre corpus principal était suffisamment grand pour prendre en charge un modèle linguistique complet.

Le point culminant de ces résultats BLEU est le score de 53,5 sur un texte mathématique (le « code linéaire » corpus). C’est beaucoup plus élevé que l’état de l’art pour la traduction automatique de l’anglais général vers le français, soit 41,8, comme atteint par le « gros » Modèle de transformateur [21]. Nous notons que lors de la traduction du « code linéaire » corpus, le système PolyMath utilise le modèle Transformer NMT pour 74% des phrases, et utilise le « système de sauvegarde » de Google Translate avec glossaire personnalisé pour les 26% restants des phrases.

TABLE 1: Résultats des tests sur deux corpus retenus : scores BLEU pour (i) le « tester » sous-ensemble de notre corpus principal multi-domaines (rangée du haut) ; et (ii) le « code linéaire » corpus composé entièrement de texte mathématique (rangée du bas). Les colonnes correspondent à : (i) Google Translate ; (ii) le modèle Transformer formé dans cet article ; (iii) puis tout le système PolyMath Translator.

|                        | Google | Transformateur | Esprit universel |
|------------------------|--------|----------------|------------------|
| texte multi-domaine    | 27,7   | 29,0           | <b>32,1</b>      |
| texte de mathématiques | 46,5   | 50,4           | <b>53,5</b>      |

**Definition 2.1.** Let  $x \in \mathbb{F}^n$ . The closed ball of radius  $r$  centered at  $x$  is defined as

$$S_r(x) = \{y \in \mathbb{F}^n \mid d(x, y) \leq r\}$$

Anglais original Latex :

Google Traduction :  
Soit  $x$  dans  $\mathbb{F}^n$ .

---

**Definition 2.1.** Let  $x \in \mathbb{F}^n$ . The closed ball of radius  $r$  centered at  $x$  is

$$S_r(x) = \{y \in \mathbb{F}^n \mid d(x, y) \leq r\}.$$

Anglais originalLatex :

```
La \ define {boule fermée de rayon $ r $
centrée sur $ x $} est
$$
S_r(x) = \{y \in \mathbb{F}^n \mid d(x, y) \leq r\}.
$$
\ end {defn}
```

**Definition 2.1.** Soit  $x \in \mathbb{F}^n$ . La boule fermée de rayon  $r$  centrée sur  $x$  est

$$S_r(x) = \{y \in \mathbb{F}^n \mid d(x, y) \leq r\}.$$

Sortie PolyMathLatex :

---

Enfin, dans le tableau [tab : texexcerpt] nous illustrons que le Polymath Le traducteur est un LaTeX système de traduction de documents, intégrant le langage naturel traduction avec analyse de documents LaTeX et prise en charge de la langue française.

La totalité de LaTeX documents sources utilisés dans cette étude, ainsi que le présent manuscrit sous forme de pré-impression, ont été traduits en français par le système PolyMath Translator, et les résultats compilés au format PDF en utilisant TeXShop ou Overleaf. La plupart des documents de sortie compilés au format PDF sans aucune modification manuelle requise. La version traduite du présent manuscrit sous forme de pré-impression est incluse dans le matériel supplémentaire, compilé au format PDF ; il s'agit de la sortie du traducteur PolyMath, avec des modifications manuelles mineures apportées à seulement 6 lignes du fichier de sortie (principalement lié aux chiffres). Il existe de légères différences de format entre l'original manuscrit et la version française, en raison du pandoc interne représentation (l'arbre syntaxique abstrait) n'étant pas une représentation parfaite de LaTeX contribution. Cependant, le le formatage est très similaire à celui du papier d'origine et le La traduction de l'anglais vers le français est très bonne.

## 4 Discussion

Nous avons mis en place un prototype de système de traduction automatique pour LaTeX documents contenant du texte mathématique. La mise en œuvre actuelle traduit l'anglais LaTeX au français LaTeX, atteignant un score BLEU de 53,5 sur un corpus de test de phrases mathématiques. Nos principales contributions sont : (i) un algorithme d'analyse LaTeX documents en phrases contenant des jetons mathématiques (en utilisant pandoc) et interagir avec les traducteurs de langue naturelle existants ; (ii) un modèle de traducteur basé sur Transformer formé (en utilisant OpenNMT) sur un corpus hétérogène contenant une petite

proportion de phrases spécifiques au domaine ; (iii) le système PolyMath Translator, qui intègre les deux éléments précédents et utilise Google Traduction avec un glossaire personnalisé comme sauvegarde. Ce système est disponible en tant que service Web à `polymathtrans.ai`.

Dans la plupart de nos expériences, nous avons constaté que la sortie de PolyMath compilée au format PDF sans erreur ni édition manuelle ; donc PolyMath est robuste dans sa gestion deLaTeXsyntaxe. Cependant PolyMath dépend du convertisseur pandoc, qui ne peut pas représenter tous les aspects de LaTeX et de ses personnalisations (par exemple les nouvelles commandes), et ainsi la sortie de PolyMath change toujours quelque peu la LaTeXsource, d'autant plus quand de nombreuses personnalisations sont utilisées. Nous nous attendons donc à ce que PolyMath soit le plus utile avec des documents dans des formats standard plus simples.

Notre score BLEU de 53,5 sur un texte mathématique est beaucoup plus élevé que l'état de l'art pour traduction automatique de l'anglais général vers le français, soit 41,8, atteint par le « gros » Modèle de transformateur[21]. Cependant, nous avons obtenu un score BLEU inférieur de 32,1 sur notre corpus principal multi-domaines (29.0 en utilisant uniquement le modèle Transformer), plus conforme aux attentes, d'autant plus que nous utilisé le « modèle de base » Transformateur et formé uniquement pendant 12 heures sur 8 V100, tandis que le résultat de pointe de 41,8 requis formation un « gros » Modèle de transformateur pendant 3 jours sur 8 V100.

Comparaison de nos résultats BLEU pour les deux corpus de test : 32.1 pour le texte multi-domaine vs. 53,5 sur un texte mathématique ; nous concluons que, puisque nous avons utilisé le même système de traduction, notre score accru sur le texte mathématique est en raison de la relative simplicité de ce domaine. En effet, alors que « simplicité » a de nombreux aspects, nous avons vérifié un aspect important : le vocabulaire de notre sous-ensemble de phrases mathématiques du corpus OPUS Wikipedia était d'environ la moitié du vocabulaire des autres sous-ensembles du même corpus de même taille, comme indiqué dans la section 2.1. Cela confirme les preuves anecdotiques et les observations[26], qui ont été notées dans l'introduction. Il serait intéressant d'étudier cela plus avant et de comparer le domaine mathématique avec d'autres domaines à cet égard. Étant donné que le texte mathématique a un vocabulaire plus petit que le langage naturel général, il offre une possibilité intrigante de traduction automatique meilleure que d'habitude, et d'autres traitements du langage naturel, dans ce domaine limité, comme le suggère notre Score BLEU de 53,5 sur un corpus de test, en utilisant un système de traduction prototype qui a une marge d'amélioration évidente.

Nous avons l'intention de développer davantage ce système. Plusieurs opportunités évidentes existent pour amélioration. Nous pouvons étendre et améliorer nos corpus et notre glossaire, en utilisant les deux outils automatisés, par exemple l'extraction automatique de terminologie multi-mots[24, 22]et relecture manuelle. Cela peut impliquer l'utilisation de grandes collections de documents, y compris arXiv, qui inclut certaines sources LaTeX accessibles au public, voir[4]. Nous pouvons intégrer les progrès récents de la recherche en tra-

duction automatique dans des domaines tels que l'apprentissage profond[28, 15], Modélisation bayésienne[27], et méthodes pour incorporer tout le contexte du document[11].

Nous étudierons également des méthodes alternatives d'analyse LaTeX qui nous permettront pour conserver exactement toutes les commandes LaTeX dans le document d'origine, plutôt que en les passant par la représentation interne de pandoc, ce qui introduit quelques changements comme mentionné ci-dessus.

Une possibilité intrigante propre au domaine du texte mathématique est d'améliorer les traductions par une compréhension sémantique contenu des formules mathématiques, voir par ex. [9]. Un objectif précoce plus simple serait classer les formules par leurs parties de discours, généralement des noms, des pronoms ou des clauses ; et les encoder d'une manière utilisable par la traduction modules.

Nous avons l'intention de prendre en charge d'autres paires de langues dans un proche avenir. De plus, étant donné la relative facilité de la traduction automatique dans le domaine du texte mathématique, comme indiqué ci-dessus, et en même temps, le manque de corpus curés de paires de phrases mathématiques, nous sommes optimistes que semi-supervisé Traduction[2]et modèles multilingues[6] réussira dans ce domaine.

## Références

- [1] Denny Britz, Quoc Le, and Reid Pryzant. Effective domain mixing for neural machine translation. In *Proceedings of the Second Conference on Machine Translation*, pages 118–126, 2017.
- [2] Yong Cheng. Semi-supervised learning for neural machine translation. In *Joint Training for Neural Machine Translation*, pages 25–40. Springer, 2019.
- [3] Chenhui Chu and Rui Wang. A survey of domain adaptation for neural machine translation. In *Proceedings of the 27th International Conference on Computational Linguistics*, pages 1304–1319, 2018.
- [4] Colin B Clement, Matthew Bierbaum, Kevin P O’Keeffe, and Alexander A Alemi. On the use of arxiv as a dataset. *arXiv preprint arXiv :1905.00075*, 2019.
- [5] Alberta Education. Lexique de mathématiques. <https://education.alberta.ca/media/481794/en-lexique-math-juillet2015.pdf>.
- [6] Orhan Firat, Kyunghyun Cho, and Yoshua Bengio. Multi-way, multilingual neural machine translation with a shared attention mechanism. *arXiv preprint arXiv :1601.01073*, 2016.
- [7] Ulrich Germann. Aligned Hansards of the 36th Parliament of Canada, Release 2001-1a. <https://www.isi.edu/natural-language/download/hansard>.

- [8] Guillaume Klein, Yoon Kim, Yuntian Deng, Jean Senellart, and Alexander Rush. OpenNMT : Open-source toolkit for neural machine translation. In *Proceedings of ACL 2017, System Demonstrations*, pages 67–72, Vancouver, Canada, July 2017. Association for Computational Linguistics.
- [9] Giovanni Yoko Kristianto, Akiko Aizawa, et al. Extracting textual descriptions of mathematical expressions in scientific papers. *D-Lib Magazine*, 20(11) :9, 2014.
- [10] Shiu-Chang Loh, Luan Kong, and Hing-Sum Hung. *Machine Translation of Chinese mathematical articles*. Department of Computer Science, 1978.
- [11] Valentin Macé and Christophe Servan. Using whole document context in neural machine translation. *arXiv preprint arXiv :1910.07481*, 2019.
- [12] John MacFarlane. Pandoc universal document converter. <https://pandoc.org/>.
- [13] Makoto Nagao, Jun ?ichi Tsujii, Koji Yada, and Toshihiro Kakimoto. An english japanese machine translation system of the titles of scientific and engineering papers. In *Coling 1982 : Proceedings of the Ninth International Conference on Computational Linguistics*, 1982.
- [14] Kishore Papineni, Salim Roukos, Todd Ward, and Wei-Jing Zhu. Bleu : a method for automatic evaluation of machine translation. In *Proceedings of the 40th annual meeting of the Association for Computational Linguistics*, pages 311–318, 2002.
- [15] Martin Popel, Marketa Tomkova, Jakub Tomek, Łukasz Kaiser, Jakob Uszkoreit, Ondřej Bojar, and Zdeněk Žabokrtský. Transforming machine translation : a deep learning system reaches news translation quality comparable to human professionals. *Nature communications*, 11(1) :1–15, 2020.
- [16] Eric Reyssat. Traduction de quelques termes mathématiques. <https://perso.crans.org/besson/publis/dicoAF.html>.
- [17] Fritz Schweiger. The grammar of mathematical symbolism. In *Evelyne Barbin, Nad'a Stehlíková und Constantinos Tzanakis eds History and Epistemology in Mathematics Education. Proceedings of the 5th European Summer University*, pages 423–430. Vydavatelství servis, 2008.
- [18] American Mathematical Society. Mathscinet mathematical reviews. <https://mathscinet.ams.org/>.
- [19] Ayla Rigouts Terryn, Véronique Hoste, and Els Lefever. In no uncertain terms : a dataset for monolingual and multilingual automatic term extraction from comparable corpora. *Language Resources and Evaluation*, pages 1–34, 2019.
- [20] Jörg Tiedemann. Parallel data, tools and interfaces in opus. In *Lrec*, volume 2012, pages 2214–2218, 2012.
- [21] Ashish Vaswani, Noam Shazeer, Niki Parmar, Jakob Uszkoreit, Llion Jones, Aidan N Gomez, Łukasz Kaiser, and Illia Polosukhin. Attention is all you need. In *Advances in neural information processing systems*, pages 5998–6008, 2017.

- [22] Branislava Šandrih, Cvetana Krstev, and Ranka Stanković. Two approaches to compilation of bilingual multi-word terminology lists from lexical resources. *Natural Language Engineering*, 26(4) :455–479, 2020.
- [23] Qingxiang Wang, Chad Brown, Cezary Kaliszyk, and Josef Urban. Exploration of neural machine translation in autoformalization of mathematics in mizar. In *Proceedings of the 9th ACM SIGPLAN International Conference on Certified Programs and Proofs*, pages 85–98, 2020.
- [24] Krzysztof Wołk and Krzysztof Marasek. Building subject-aligned comparable corpora and mining it for truly parallel sentence pairs. *Procedia Technology*, 18 :126–132, 2014.
- [25] Magdalena Wolska, Mihai Grigore, and Michael Kohlhase. Using discourse context to interpret object-denoting mathematical expressions. In *Proc. of the CICM Workshop DML-11*, pages 85–101. Masaryk University Press (Brno, Czech Republic), 2011.
- [26] Taha Yasseri, András Kornai, and János Kertész. A practical approach to language complexity : a wikipedia case study. *PloS one*, 7(11) :e48386, 2012.
- [27] Lei Yu, Laurent Sartran, Wojciech Stokowiec, Wang Ling, Lingpeng Kong, Phil Blunsom, and Chris Dyer. Better document-level machine translation with Bayes’ rule. *Transactions of the Association for Computational Linguistics*, 8 :346–360, 2020.
- [28] Biao Zhang, Deyi Xiong, Jun Xie, and Jinsong Su. Neural machine translation with GRU-gated attention model. *IEEE Transactions on Neural Networks and Learning Systems*, 2020.
